# Supplementary material for: DyFormer: A Scalable Dynamic Graph Transformer with Provable Benefits on Generalization Ability
Source: arXiv:2111.10447 source file (2023-01-30)
Supplement: Supplementary file 1 [file dataset_stat.tex]

\subsection{Details on datasets}\label{section:dataset_details}

We summarize the dataset statistic in Table~\ref{table:dataset_stat}.
More specifically, we prepare snapshot graphs following the procedure as described in~\cite{sankar2018dynamic}.
In the following, we provide brief descriptions of each dataset.

\begin{itemize} [noitemsep,topsep=0pt,leftmargin=3mm ]
\item\textbf{Enron dataset}\footnote{\url{https://www.cs.cmu.edu/~enron/}}: Enron is a public available social network dataset which contains data from about $150$ users. We only consider the email communications between Enron employees to generate the dynamic dataset, and use a $2$ month sliding window to construct $16$ snapshots.

\item\textbf{RDS dataset}\footnote{\url{https://nrvis.com/download/data/dynamic/ia-radoslaw-email.zip}}: This is a publicly available social network dataset that contains an email communication network between employees of a mid-sized manufacturing company Radoslaw. Nodes represent employees and edges represent individual emails between two users. The snapshots are created using a window size of $3$ days.

\item\textbf{UCI dataset}\footnote{\url{http://konect.cc/networks/opsahl-ucsocial/}}: This is a publicly available social network dataset that contains private messages sent between users on an online social network platform at the University of California, Irvine over $6$ months. The snapshots are created using a window size of $10$ days.

\item\textbf{Yelp dataset}\footnote{\url{https://www.yelp.com/dataset}}: This is a public available rating dataset which contains user-business rating in Arizona. We only consider user-business pairs that have at least $15$ interactions. The snapshots are created using a window size of $6$ months.

\item\textbf{ML-10M}\footnote{\url{https://grouplens.org/datasets/movielens/10m/}}: This is a publicly available rating dataset that contains tagging behavior of MovieLens users, with the tags applied by a user on her rated movies. The snapshots are created using a window size of $3$ months.

\item\textbf{Wikipedia}\footnote{\url{http://snap.stanford.edu/jodie/wikipedia.csv}}: This is a publicly available interaction graph, where users and pages are nodes, and an interaction represents a user editing a page. The snapshots are created using a window size of $3$ days.

\item\textbf{Reddit}\footnote{\url{http://snap.stanford.edu/jodie/reddit.csv}}: This is a publicly available interaction graph, where users and subreddits are nodes, and interaction occurs when a user writes a post to the subreddit. The snapshots are created using a window size of $3$ days. The data is from a pre-existing, publicly available dataset collected by a third party.
\end{itemize}

\subsection{Details on datasets}\label{section:dataset_details}

We summarize the dataset statistic in Table~\ref{table:dataset_stat}.
More specifically, we prepare snapshot graphs following the procedure as described in~\cite{sankar2018dynamic}.
In the following, we provide brief descriptions of each dataset.

\begin{itemize} [noitemsep,topsep=0pt,leftmargin=3mm ]
\item\textbf{Enron dataset}\footnote{\url{https://www.cs.cmu.edu/~enron/}}: Enron is a public available social network dataset which contains data from about $150$ users. We only consider the email communications between Enron employees to generate the dynamic dataset, and use a $2$ month sliding window to construct $16$ snapshots.

\item\textbf{RDS dataset}\footnote{\url{https://nrvis.com/download/data/dynamic/ia-radoslaw-email.zip}}: This is a publicly available social network dataset that contains an email communication network between employees of a mid-sized manufacturing company Radoslaw. Nodes represent employees and edges represent individual emails between two users. The snapshots are created using a window size of $3$ days.

\item\textbf{UCI dataset}\footnote{\url{http://konect.cc/networks/opsahl-ucsocial/}}: This is a publicly available social network dataset that contains private messages sent between users on an online social network platform at the University of California, Irvine over $6$ months. The snapshots are created using a window size of $10$ days.

\item\textbf{Yelp dataset}\footnote{\url{https://www.yelp.com/dataset}}: This is a public available rating dataset which contains user-business rating in Arizona. We only consider user-business pairs that have at least $15$ interactions. The snapshots are created using a window size of $6$ months.

\item\textbf{ML-10M}\footnote{\url{https://grouplens.org/datasets/movielens/10m/}}: This is a publicly available rating dataset that contains tagging behavior of MovieLens users, with the tags applied by a user on her rated movies. The snapshots are created using a window size of $3$ months.

\item\textbf{Wikipedia}\footnote{\url{http://snap.stanford.edu/jodie/wikipedia.csv}}: This is a publicly available interaction graph, where users and pages are nodes, and an interaction represents a user editing a page. The snapshots are created using a window size of $3$ days.

\item\textbf{Reddit}\footnote{\url{http://snap.stanford.edu/jodie/reddit.csv}}: This is a publicly available interaction graph, where users and subreddits are nodes, and interaction occurs when a user writes a post to the subreddit. The snapshots are created using a window size of $3$ days. The data is from a pre-existing, publicly available dataset collected by a third party.
\end{itemize}
