# Supplementary material for: DyFormer: A Scalable Dynamic Graph Transformer with Provable Benefits on Generalization Ability
Source: arXiv:2111.10447 source file (2023-01-30)
Supplement: Supplementary file 2 [file more_experiments.tex]

\section{More experiment results}\label{section:more_experiments}
% ~\yh{Can you add some text description (e.g., introduce the settings) to each of the sub appendix and table?}

\subsection{Link prediction results}\label{section:link_pred_appendix}
In this section, we provide the remained figures and tables in Section~\ref{section:experiments}. 

\noindent\textbf{Comparison of AUC score at different time steps.}~
In Figure~\ref{fig:time_step_curve}, we compare the AUC score of \our with baselines on Enron, UCI, Yelp, and ML-10M dataset. We can observe that \our can consistently outperform baselines on Enron and ML-10M dataset at all time steps, but has a relatively lower AUC score at certain time steps on the UCI and Yelp dataset. Besides, the performance of \our is relatively more stable than baselines on different time steps.

\begin{figure}[h]
    \centering
    \includegraphics[width=.9\textwidth]{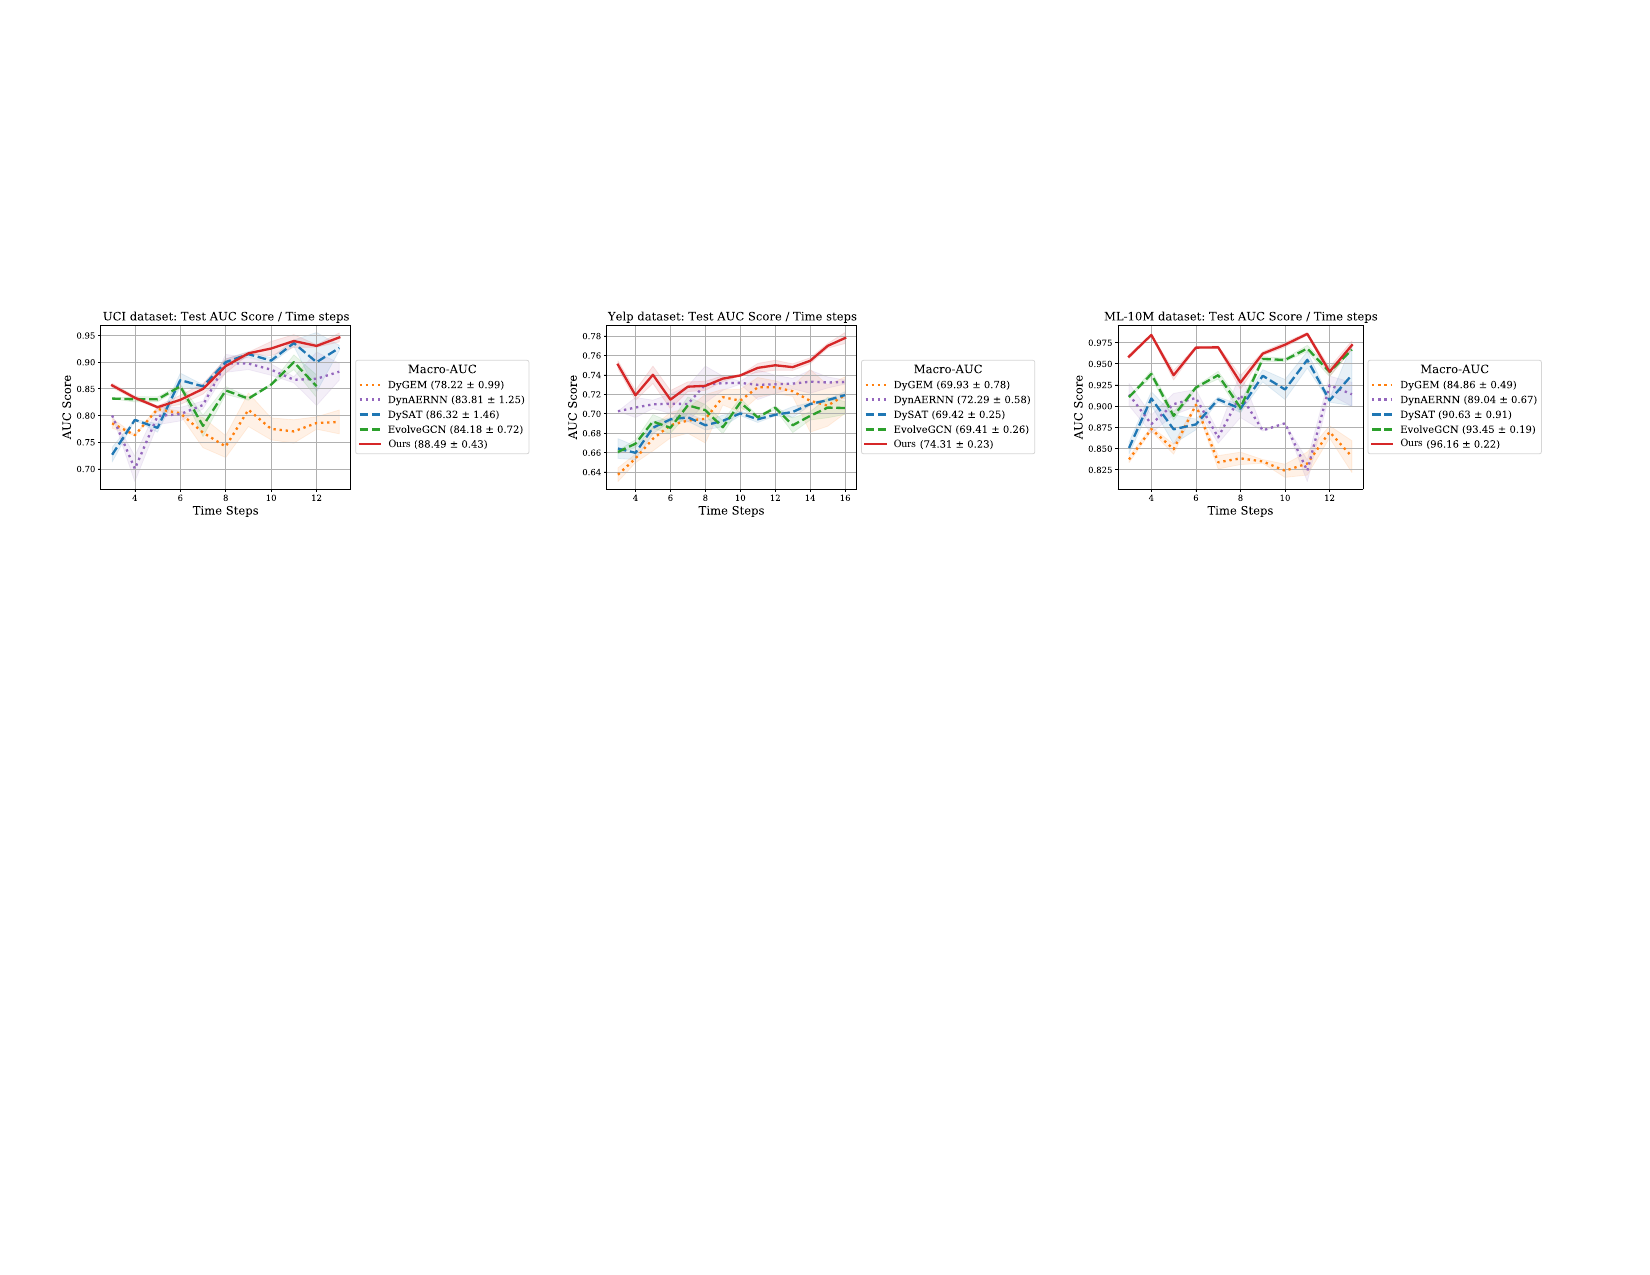}
    \vspace{-10pt}
    \caption{Comparison of \our with baselines across multiple time steps, where the Macro-AUC score is reported in the box next to the curves.}
    \label{fig:time_step_curve}
\end{figure}

\noindent\textbf{Comparision of AUC score on new link prediction task.}~
In Table~\ref{table:single_step_link_prediction_new_edge}, we report dynamic link prediction result evaluated only on the new links at each time step, where a link that appears at the current snapshot but not in the previous snapshot is considered as a new link. This experiment can provide an in-depth analysis of the capabilities of different methods in predicting unseen links. 
As shown in Table~\ref{table:single_step_link_prediction_new_edge}, all methods achieve a lower AUC score, which is expected because new link prediction is more challenging. However, \our still achieves consistent  gains of $1\sim 3\%$ Macro-AUC over baselines,
thus illustrate its effectiveness in accurately temporal context for new link prediction.

\input{sections/tables/compare_to_baseline_new_edge}

\clearpage

\noindent\textbf{Computation time and memory consumption.}~
In Table~\ref{table:memory_time}, we compare the memory consumption and epoch time on the last time step of ML-10M and Yelp dataset. We chose the last time step of these two datasets because its graph size is relatively larger than others, which can provide a more accurate time and memory estimation. The memory consumption is record by  \texttt{nvidia-smi} and the time is recorded by function \texttt{time.time()}. During pre-training, \our samples $256$ context node and $256$ context node at each iteration. During fine-tuning, \our first $256$ positive links (links in the graph) and sample $2,560$ negative links (node pairs that do not exist in the graph), then treat all nodes in the sampled node pairs at target nodes and sample the same amount of context nodes. Notice that although the same sampling size hyper-parameter is used, since the graph size and the graph density are different, the actual memory consumption and time are also different. 
% Besides, since PyTorch is using use a caching allocator to speed up training, therefore the reported memory consumption is more than it actually required. In practice, we also test \our with the same setting 
For example, since the Yelp dataset has more edges with more associated nodes for evaluation than ML-10M, the memory consumption and time are required on Yelp than on ML-10M dataset.
\input{sections/tables/memory_time}

\subsection{Ablation study results.} \label{section:ablation_study_appendix}
In this section, we provide missing the tables in Section~\ref{section:ablation_study}, where  discussion on the results are provided in Section~\ref{section:ablation_study}.

%########################################################
%########################################################
%########################################################
\noindent\textbf{Compare two-tower to single-tower architecture.}~
In Table~\ref{table:single_two_tower},  we compare the Micro-AUC score and Macro-AUC score of \our with one-tower\footnote{The node representation  $\mathbf{H}^{(\ell)}$  in the single-tower \our is computed by
\begin{equation}
    \begin{aligned}
    \mathbf{H}^{(\ell)} &= \textit{FFN}(\textit{LN}(\mathbf{Z}^{(\ell)} )) + \mathbf{Z}^{(\ell)} \\
    \mathbf{Z}^{(\ell)} &= \textit{Softmax} \left( \frac{(\textit{LN}( \mathbf{H}^{(\ell-1)} )\mathbf{W}_Q^{(\ell)} ) (\textit{LN}(\mathbf{H}^{(\ell-1)}) \mathbf{W}_K^{(\ell)} )^\top  }{\sqrt{d}} + \mathbf{A}_\text{TC} + \mathbf{A}_\text{SD} \right)\textit{LN}(\mathbf{H}^{(\ell-1)}) \mathbf{W}_V^{(\ell)}  + \mathbf{H}^{(\ell-1)}.
    \end{aligned}
\end{equation}
} and two-tower structure on UCI, Yelp, and ML-10M datasets.
% Recall that  nodes within target node set and context node set are sampled independently but there exist neighborhood relationships between inter-group nodes. 
% Only attending inter-group nodes help \our better capturing these context information without fusing representations from irrelevant nodes.
% To see this, we compare the performance of \our using single-tower and two tower. 
% As shown in Table~\ref{table:single_two_tower}, two-tower structure enjoys a consistent performance gain over the single-tower structure on all datasets.
\input{sections/tables/compare_1_tower_vs_2_tower}

%########################################################
%########################################################
%########################################################

\clearpage
%########################################################
%########################################################
%########################################################
\noindent\textbf{Compare $K$-hop attention with full attention.}~
In Table~\ref{table:single_two_tower}, we compare the performance of ``single-tower \our using full-attention'', ``single-tower \our using $1$-hop attention'', and ``single-tower \our using $3$-hop attention'' on the UCI, Yelp, and ML-10M dataset. 
% The classical GNNs over-rely on the fixed graph structure, a noisy graph with missing or spurious connections may lead to poor performance. We overcome this by leveraging the idea of full attention in Transformers. By doing so, \our can capture the implicit edge connections in the graph and have a relatively larger receptive field comparing to its $K$-hop counterparts.
% To see this, we compare the performance of single-tower \our using full-attention with $1$-hop and $3$-hop attention.
% Here we use single-tower to eliminate the effect of two-tower message passing.
% As shown in Table~\ref{table:single_two_tower}, the full-attention enjoys a consistent performance gain over its $1$-hop and $3$-hop attention counterparts.

\input{sections/tables/compare_k_hop_vs_full_attention}

%########################################################
%########################################################
%########################################################

\noindent\textbf{The effectiveness of spatial-temporal encoding.}~
In Table~\ref{table:compare_positional_encoding}, we validate the effectiveness of spatial-temporal encoding by independently removing the temporal edge coding and spatial distance encoding.
% To validate the effectiveness of spatial-temporal encoding, we conduct an ablation study by independently removing the temporal edge coding and spatial distance encoding.
% From Table~\ref{table:compare_positional_encoding}, we observe that even without spatial-temporal encoding (i.e., ignore graph topology), due to full attention, \our can still learn the graph structure by optimizing the graph structure reconstruction loss. However, better performance can be achieved by providing \our the graph topology information using spatial-temporal encoding.

\input{sections/tables/compare_positional_encoding}

%########################################################
%########################################################
%########################################################

\noindent\textbf{The effect of the number of layers.}~
In Table~\ref{table:number_of_layers}, we compare the Micro-AUC score and Macro-AUC score of \our with a different number of layers on the UCI, Yelp, and ML-10M datasets.
% In classical GNNs, each individual layers only consider the local interactions. To model longer-range dependencies, GNNs require a deep architecture so that information can be propagated from distant nodes. Deep GNNs usually suffer from over-smoothing and bottleneck effects, which results in a degenerated performance.
% Comparing to GNNs, our model only requires a shallow architecture because each individual layer is capable of modeling longer-range dependencies. Besides, the self-attention mechanism can automatically attend to important neighbors, therefore alleviate the over-smoothing and bottleneck effect in GNNs.
% As shown in Table~\ref{table:number_of_layers}, the performance of our model with a different number of layers is relatively stable and does not show the phenomenon of performance degradation as the number of model layers increases.

\input{sections/tables/compare_diff_layers}

% ML-10M dataset for finial time step prediction
% EvolveGCN epoch time 6.9s 13.6G memory --- Two-layer model, but requires full-batch training
% 

% \clearpage

% \weilin{
% Compare with baselines
% \begin{itemize}
%     \item \st{(Done, but need to plot it) Single-step prediction under transduction learning setting without node feature. Datasets (x5): UCI, Enron, , RDS, Yelp, ML-10M.}
%     \item Single step prediction under inductive learning setting with node feature
%     \item Node classification: working on it, expect to finish by Wednesday
%     \item \st{Edge classification: TBD }
%     \item Complexity analysis?
% \end{itemize}
% }

% \weilin{Ablation study:
% \begin{itemize}
%     \item \st{(In progress) Compare with and without pre-training (with different pre-training tasks)}
%     \item \st{(In progress) shallow v.s. deep layers for oversmoothing? }
%     \item \st{Compare one-tower to two tower}
%     \item Compare with and without edge encoding, Compare with and without distance encoding
%     \item \st{Compare full attention vs k-hop attention}
%     \item \st{(no need) Compare with and without temporal weight}
%     \item (less important) Compare different ways of generating common neighbor
% \end{itemize}
% }

\clearpage
\subsection{Node classification results} \label{section:node_cls}
In this section, we show that although \our is orginally designed for the link prediction task, the learned representation of \our can be also applied to binary node classification.
We evaluate \our on Wikipedia and Reddit dataset, where dataset statistic is summarized in Table~\ref{table:dataset_stat}.
The snapshot is created in a similar manner as the link prediction task.
% Similar to the link prediction task, snapshot graphs are created by splitting the data using suitable time windows such that each snapshot has an equitable and reasonable number of interactions. In each snapshot, the edge weight is determined by the number of interactions between the associated node pairs during that time duration.
As shown in Table~\ref{table:node_cls} and Figure~\ref{fig:node_cls}, \our performs around $0.7\%$ better than all baselines on the Wikipedia dataset and around $0.7\%$ better than \textsc{EvolveGCN} on Reddit dataset. However, the results \our on the Reddit dataset is slightly lower than \textsc{DySAT}. This is potentially due to \our is less in favor of a dense graph, e.g., Reddit dataset, with very dense graph structure information encoded by spatial-temporal encodings.

\input{sections/tables/node_classification}

\begin{figure}[h]
    \centering
    \includegraphics[width=0.99\textwidth]{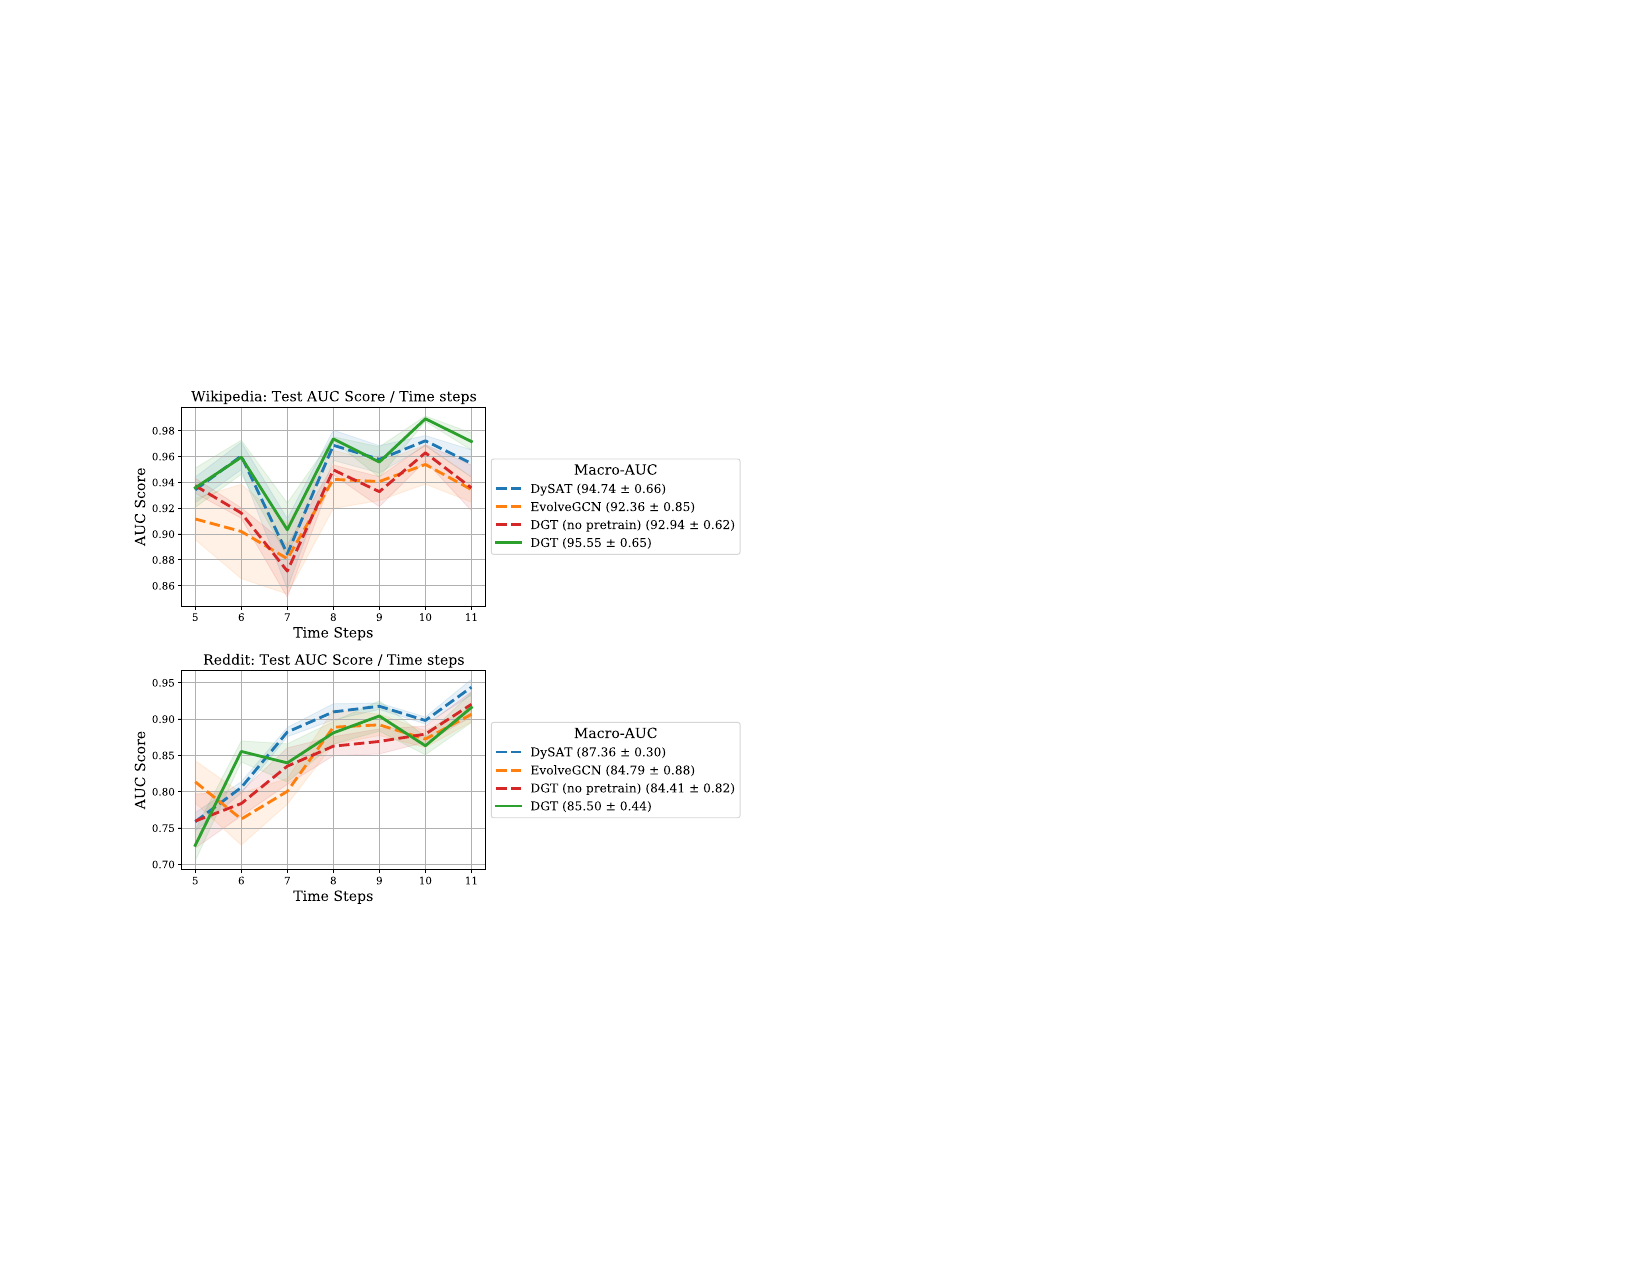}
    \vspace{-10pt}
    \caption{Comparison of \our with baselines across multiple time steps, where the Macro-AUC score is reported in the box next to the curves}
    \label{fig:node_cls}
\end{figure}

\subsection{Results on noisy dataset}
In this section, we study the effect of noisy input on the performance of \our using \textit{UCI} and \textit{Yelp} datasets. We achieve this by randomly selecting $10\%$, $20\%$, $50\%$ of the node pairs and changing their connection status either from connected to not-connected or from not-connected to connected. 
As shown in Table~\ref{eq:noisy_input}, although the performance of both using full-attention and 1-hop attention decreases as the noisy level increases, the performance of using full-attention aggregation is more stable and robust as the noisy level changes. 
This is because 1-hop attention relies more on the given structure, while full-attention only take the give structure as a reference and learns the ``ground truth'' underlying graph structure by gradient descent update.

% \begin{table}[h]
% \caption{Comparison of the \textit{Macro-AUC} score of \our and its variants with input graph with different noisy level.} \label{eq:noisy_input}

% \centering
% \begin{tabular}{l l c c c }
% \hline\hline
%                       & Method                      & $10\%$ & $20\%$ & $50\%$ \\ \hline\hline
% \multirow{4}{*}{\textbf{UCI}}   & \our (1-hop attention aggregation) & $83.01 \pm 0.61$ & $82.10 \pm 0.60$ & $79.95 \pm 0.67$ \\ % \cline{2-5}
%                                 & \our (Full attention aggregation)  & $86.12 \pm 0.57$ & $85.93 \pm 0.59$ & $85.51 \pm 0.51$ \\ \cline{3-5}
%                                 & \our (1-hop mean aggregation)      & $ $ & $ $ & $ $ \\
%                                 & \our (Full mean aggregation)       & $ $ & $ $ & $ $ \\ \hline
% \multirow{4}{*}{\textbf{Yelp}}  & \our (1-hop attention aggregation) & $69.94 \pm 0.20$ & $68.45 \pm 0.23$ & $65.61 \pm 0.15$ \\ % \cline{2-5}
%                                 & \our (Full attention aggregation)  & $71.64 \pm 0.18$ & $71.67 \pm 0.21$ & $69.93 \pm 0.21$ \\ \cline{3-5}
%                                 & \our (1-hop mean aggregation)      & $ $ & $ $ & $ $ \\
%                                 & \our (Full mean aggregation)       & $ $ & $ $ & $ $ \\ \hline\hline
% \end{tabular}
% \end{table}

\begin{table}[h]
\caption{Comparison of the \textit{Macro-AUC} score of \our and its variants with input graph with different noisy level.} \label{eq:noisy_input}
\centering
\begin{tabular}{ l l l c c c }
\hline\hline
                       & Method                                       &           & 10\% & 20\% & 50\% \\ \hline\hline
\multirow{4}{*}{\textbf{UCI}}    & \multirow{2}{*}{our (1-hop attention)}       & Micro-AUC & $82.97 \pm 0.56$ & $81.23 \pm 0.78$ & $77.85 \pm 0.66$ \\ % \cline{3-6} 
                                 &                                              & Macro-AUC & $83.01 \pm 0.61$ & $82.10 \pm 0.60$ & $78.43 \pm 0.67$ \\ \cline{2-6} 
                                 & \multirow{2}{*}{our (Full aggregation)}      & Micro-AUC & $86.98 \pm 0.51$ & $86.10 \pm 0.57$ & $84.36 \pm 0.49$ \\ % \cline{3-6} 
                                 &                                              & Macro-AUC & $86.12 \pm 0.57$ & $85.93 \pm 0.59$ & $85.51 \pm 0.51$ \\ \hline
\multirow{4}{*}{\textbf{Yelp}}   & \multirow{2}{*}{our (1-hop attention)}       & Micro-AUC & $70.00 \pm 0.20$ & $68.55 \pm 0.21$ & $65.32 \pm 0.22$ \\ % \cline{3-6} 
                                 &                                              & Macro-AUC & $69.94 \pm 0.20$ & $68.45 \pm 0.23$ & $65.61 \pm 0.15$ \\ \cline{2-6} 
                                 & \multirow{2}{*}{our (Full aggregation)}      & Micro-AUC & $70.99 \pm 0.20$ & $71.74 \pm 0.19$ & $70.93 \pm 0.21$ \\ % \cline{3-6} 
                                 &                                              & Macro-AUC & $71.64 \pm 0.18$ & $71.67 \pm 0.21$ & $69.93 \pm 0.21$ \\ \hline\hline
\end{tabular}
\end{table}

%########################################################
%########################################################
%########################################################
\subsection{Comparison with continuous-graph learning algorithms}
In this section, we compare snapshot graph-based methods against continuous graph-based learning algorithm on the \textit{UCI}, \textit{Yelp}, and \textit{ML-10M} dataset. For the continuous graph learning algorithm, we choose
% \href{https://github.com/srijankr/jodie}{JODIE}
JODIE~\cite{kumar2019predicting} and 
% \href{https://github.com/StatsDLMathsRecomSys/Inductive-representation-learning-on-temporal-graphs}{TGAT}
TGAT~\cite{xu2020inductive} as the baseline. As shwon in Table~\ref{table:cont_method}, JODIE and TGAT suffer from significant performance degradation. This is because they are designed to leverage the edge features and fine-grained timestamp information for link prediction, however, these information is lacking on existing snapshot graph datasets.

Please note that we compare with continuous graph algorithm only for the sake of completeness. However, since snapshot graph-based methods and continuous graph-based methods require different input graph structures, different evaluation strategies, and are designed under different settings, directly comparing two sets of methods cannot provide much meaningful interpretation.
For example, existing works~\cite{kumar2019predicting,xu2020inductive} on a continuous graph select the training and evaluation set by taking the first $80\%$ of links in the dataset for training and taking the rest for evaluation. In other words, the training and evaluation samples can be arbitrary close and might even come from the same time step. However, in the snapshot graph, the training and evaluation set is selected by taking the links in the previous $T-1$ snapshot graphs for training and evaluating on the $T$-th snapshot graph. That is, the training and evaluation samples never come from the same time step. Besides, since the time steps in the continuous graph are fine-grained than snapshot graphs, continuous graph methods suffer from performance degradation when applied on the snapshot graph dataset due to lack of fine-grained timestamp information.
Due to the aforementioned reasons, existing continuous graph learning methods (e.g., Jodie, TGAT) only compare with other continuous graph methods on the continuous datasets, similarly, existing snapshot graph learning methods (e.g., DySAT, EvolveGCN, DynAERNN, DynGEM) also only considers other snapshot graph based methods as their baseline for a comparison.

\begin{table}[h]
\centering
\caption{Comparison of the \textit{Micro}- and \textit{Macro}-\textit{AUC} score of \DGT, JODIE on the real-world datasets.
% , where ``$-$'' stands for the code is not runable due to more than $24$GB GPU memory is required during training.
} \label{table:cont_method}
\scalebox{0.99}{
\begin{tabular}{llccc}
\hline\hline
\textbf{Method}                & \textbf{Metric}    & \textbf{UCI}        & \textbf{Yelp}        & \textbf{ML-10M}     \\ \hline\hline

\multirow{2}{*}{\DGT}    & \text{Micro-AUC}   & $\bm{87.91\pm0.32}$      & $\bm{ 73.39 \pm 0.21}$      & $ \bm{95.30 \pm 0.36}$     \\ % \cline{2-8} 
                         & \text{Macro-AUC}   & $\bm{88.49\pm0.43}$      & $\bm{ 74.31 \pm 0.23}$      & $ \bm{96.16 \pm 0.22}$     \\ \hline
\multirow{2}{*}{JODIE}   & \text{Micro-AUC}   & $57.99\pm0.34$           & $ 59.85 \pm 0.32 $          & $ 62.84 \pm 0.47$          \\ % \cline{2-8} 
                         & \text{Macro-AUC}   & $57.21\pm0.37$           & $61.01\pm 0.44$             & $ 61.30 \pm 0.46 $         \\ \hline
\multirow{2}{*}{TGAT}    & \text{Micro-AUC}   & $ 48.15 \pm 0.45$        & $ 51.95 \pm 0.39$           & $ 52.15 \pm 0.51$          \\ % \cline{2-8} 
                         & \text{Macro-AUC}   & $ 49.02 \pm 0.43$        & $ 52.78 \pm 0.40$           & $ 51.15 \pm 0.50$          \\ \hline\hline
\end{tabular}
}
% \vspace{-5pt}
\end{table}
