# Supplementary material for: DyFormer: A Scalable Dynamic Graph Transformer with Provable Benefits on Generalization Ability
Source: arXiv:2111.10447 source file (2023-01-30)
Supplement: Supplementary file 3 [file multiview_landscape.tex]

\section{Why multi-view pre-training objective work}\label{section:landscape_self_supervised}

\weilin{The multi-view loss gives us two global optima solution, $\mathbf{A}_i = \mathbf{0}$ or $\mathbf{A}_i = \mathbf{A}_i^\star \mathbf{O}$ upon convergence. $\mathbf{A}_i = \mathbf{0}$ is not what we expect. Fortunately, by introducing reconstruct loss, we can eliminate this from global optima solution candidate set.}

Let say we have $N$ linear equations: $$\mathbf{y}_i = \mathbf{A}_i \mathbf{x}, ~i\in[N],$$
where $\mathbf{y}_i \in \mathbb{R}^{d_y}, \mathbf{x}\in\mathbb{R}^{d_x}, \mathbf{A}_i \in\mathbb{R}^{d_y\times d_x}$ with $d_y\ll d_x$.

\weilin{$\mathbf{\mathbf{x}}$ is a vector that captures all the graph structure information of snapshot graps, for example $\mathbf{x} = \text{vec}(\mathbf{H}_\star^{(L)}) \in\mathbf{R}^{Nd}$, where $\mathbf{H}_\star^{(L)} \in \mathbb{R}^{N\times d}$ is the ground truth node representation (have no access but want to estimate it from data).}

\weilin{For example in link prediction task, we can define $\mathbf{y}_i$ as a vector indicate whether there exist link between node $i,j$ at time $t$, i.e., $\mathbf{y}_i = [v_i, v_j, \psi(v_i, v_j, 1), \psi(v_i, v_j, 2), \ldots, \psi(v_i, v_j, T)] \in \mathbb{R}^{2+T}$ for any $v_i, v_j \in \mathcal{V}$ and $t\in[T]$}

This can be solved by pseudo-inverse if $\det(\mathbf{A}_i^\top \mathbf{A}_i) \neq 0$ because of $\left(\mathbf{A}_i^\top \mathbf{A}_i\right)^{-1}$ requires so: $$\mathbf{x} = \left(\mathbf{A}_i^\top \mathbf{A}_i\right)^{-1} \left(\mathbf{A}_i^\top \mathbf{y}_i\right)$$
Unfortunately $\det(\mathbf{A}_i^\top \mathbf{A}_i) = 0$ because $\mathbf{A}_i$ is fat matrix with $\text{rank}(\mathbf{A}_i) = d_y < d_x$.

However, since we have $N$ such linear equations, we can estimate $\mathbf{x}$ by
$$\hat{\mathbf{x}} = \left(\sum_{i=1}^N\mathbf{A}_i^\top \mathbf{A}_i\right)^{-1} \left(\sum_{i=1}^N\mathbf{A}_i^\top \mathbf{y}_i\right) \in \mathbb{R}^{d_x}$$
because
$$
\left(\sum_{i=1}^N \mathbf{A}_i \right) \mathbf{x} = \sum_{i=1}^N \mathbf{y}_i
\Leftrightarrow \left( \sum_{i=1}^N \mathbf{A}_i^\top \mathbf{A}_i \right)\mathbf{x} = \sum_{i=1}^N \mathbf{A}_i^\top \mathbf{y}_i
$$

Instead of using all $N$ equations, we can just sample subset $\mathcal{S}$ and estimate
$$\hat{\mathbf{x}}(\mathcal{S}, \mathcal{A}) = \left(\sum_{i\in\mathcal{S}}\mathbf{A}_i^\top \mathbf{A}_i\right)^{-1} \left(\sum_{i\in\mathcal{S}}\mathbf{A}_i^\top \mathbf{y}_i\right) \in \mathbb{R}^{d_x},~\mathcal{S} \subset [N]$$

\weilin{
Do we have an upper bound on $\|\mathbf{x} - \hat{\mathbf{x}} \|_2 \leq C$ where $C$ is expected to be related to $d_x, d_y, N$? }

Let $\mathbf{M}_\varepsilon(\mathcal{S},\mathcal{A}) = \sum_{i\in\mathcal{S}} \mathbf{A}_i^\top \mathbf{A}_i + \varepsilon \mathbf{I} \in \mathbb{R}^{d_x\times d_x}$ and $\mathbf{v}(\mathcal{S},\mathcal{A}) = \sum_{i\in\mathcal{S}} \mathbf{A}_i^\top \mathbf{y}_i \in \mathbb{R}^{d_x}$, where $\mathcal{S} \subset [N]$.
Then, we have $$\hat{\mathbf{x}}(\mathcal{S},\mathcal{A}) = \left(\sum_{i\in\mathcal{S}}\mathbf{A}_i^\top \mathbf{A}_i + \varepsilon \mathbf{I} \right)^{-1} \left(\sum_{i\in\mathcal{S}}\mathbf{A}_i^\top \mathbf{y}_i\right) = \mathbf{M}_\varepsilon^{-1} (\mathcal{S},\mathcal{A})\mathbf{v}(\mathcal{S},\mathcal{A}) \in \mathbb{R}^{d_x}$$.

Let $\mathcal{A} = \{ \mathbf{A}_i \}_{i=1}^N $, $\mathbf{M}^\star(\mathcal{S},\mathcal{A}) = \sum_{i\in\mathcal{S}}\mathbf{A}_i^\top \mathbf{A}_i^\star \in \mathbb{R}^{d_x \times d_x}$, $\mathbf{A}_i^\star \in \mathbb{R}^{d_y \times d_x}$ is the ground truth weight matrix, and $\mathbf{K}(\mathcal{S},\mathcal{A}) = \mathbf{M}_\varepsilon^{-1}(\mathcal{S},\mathcal{A}) \mathbf{M}^\star (\mathcal{S},\mathcal{A}) \in \mathbb{R}^{d_x\times d_x}$.

For multi-view contrastive (let representation as close as possible), we have 
\begin{align*}
\widehat{\mathcal{A}} = & \arg\min_{\mathcal{A}} \mathcal{L}_\text{view}(\mathcal{A}) \\
& = \arg\min_{\mathcal{A}} \mathbb{E}_{\mathbf{x}, \mathcal{S}_1, \mathcal{S}_2} [\| \hat{\mathbf{x}}(\mathcal{S}_1,\mathcal{A}) - \hat{\mathbf{x}}(\mathcal{S}_2,\mathcal{A})\|_2^2] \\
&= \arg\min_{\mathcal{A}} \mathbb{E}_{\mathbf{x}, \mathcal{S}_1, \mathcal{S}_2} \left[\left\| \left(\sum_{i\in\mathcal{S}_1}\mathbf{A}_i^\top \mathbf{A}_i + \varepsilon \mathbf{I} \right)^{-1} \left(\sum_{i\in\mathcal{S}_1}\mathbf{A}_i^\top \mathbf{y}_i\right) - \left(\sum_{i\in\mathcal{S}_2}\mathbf{A}_i^\top \mathbf{A}_i + \varepsilon \mathbf{I} \right)^{-1} \left(\sum_{i\in\mathcal{S}_2}\mathbf{A}_i^\top \mathbf{y}_i\right) \right\|^2_2 \right] \\
&= \arg\min_{\mathcal{A}} \mathbb{E}_{\mathbf{x}, \mathcal{S}_1, \mathcal{S}_2} \left[\left\| \left(\sum_{i\in\mathcal{S}_1}\mathbf{A}_i^\top \mathbf{A}_i + \varepsilon \mathbf{I} \right)^{-1} \left(\sum_{i\in\mathcal{S}_1}\mathbf{A}_i^\top \mathbf{A}_i^\star \mathbf{x} \right) - \left(\sum_{i\in\mathcal{S}_2}\mathbf{A}_i^\top \mathbf{A}_i + \varepsilon \mathbf{I} \right)^{-1} \left(\sum_{i\in\mathcal{S}_2}\mathbf{A}_i^\top \mathbf{A}_i^\star \mathbf{x}  \right) \right\|^2_2 \right]\\
&= \arg\min_{\mathcal{A}} \mathbb{E}_{\mathcal{S}_1, \mathcal{S}_2} \left[\left\| \left(\sum_{i\in\mathcal{S}_1}\mathbf{A}_i^\top \mathbf{A}_i + \varepsilon \mathbf{I} \right)^{-1} \left(\sum_{i\in\mathcal{S}_1}\mathbf{A}_i^\top \mathbf{A}_i^\star \right) - \left(\sum_{i\in\mathcal{S}_2}\mathbf{A}_i^\top \mathbf{A}_i + \varepsilon \mathbf{I} \right)^{-1} \left(\sum_{i\in\mathcal{S}_2}\mathbf{A}_i^\top \mathbf{A}_i^\star  \right) \right\|^2_2 \right] \\
&= \arg\min_{\mathcal{A}} \mathbb{E}_{\mathcal{S}_1, \mathcal{S}_2} [\| \mathbf{M}_\varepsilon^{-1}(\mathcal{S}_1, \mathcal{A}) \mathbf{M}^\star (\mathcal{S}_1, \mathcal{A})- \mathbf{M}^{-1}_\varepsilon(\mathcal{S}_2, \mathcal{A}) \mathbf{M}^\star (\mathcal{S}_2, \mathcal{A})\|^2_\mathrm{F}] \\
&= \arg\min_{\mathcal{A}} \mathbb{E}_{\mathcal{S}_1, \mathcal{S}_2} [\| \mathbf{K}(\mathcal{S}_1, \mathcal{A}) - \mathbf{K}(\mathcal{S}_2, \mathcal{A})\|^2_\mathrm{F}]
\end{align*}

There  are two points that can minimize the objective
\begin{itemize}
    \item All elements in $\mathcal{A}$ are zero matrices, i.e., $\mathbf{A}_i = \mathbf{0},~\forall i\in[N]$
    \item $\mathbf{A}_i = \mathbf{P}_i \mathbf{A}_i^\star$ where $\mathbf{P}_i$ is a projection matrix with $\mathbf{P}_i = \mathbf{P}_i^\top, \mathbf{P}_i^2 = \mathbf{P}_i$.
    \item $\mathbf{A}_i = \alpha \mathbf{A}_i^*, \mathbf{A}_i = \mathbf{A}_i^\star \mathbf{M}{-1} $
    \item Each $\mathbf{A}_i $ converge to $\mathbf{A}_i^\star \mathbf{O}$, where $\mathbf{O}$ is any orthogonal matrices.
\end{itemize}

\weilin{===============================\\}

For reconstruct loss (using the estimated representation recover the graph structure) we have
\begin{equation} \label{eq:failure_loss_2}
    \begin{aligned}
    \min_{\mathcal{A}} \mathcal{L}_\text{recon}(\mathcal{A}) &= \min_{\mathcal{A}}  \mathbb{E}_{\mathbf{x}, \mathcal{S}} \left[ \sum_{j\in\mathcal{S}} \| \mathbf{y}_j - \mathbf{A}_j \hat{\mathbf{x}}(\mathcal{S}, \mathcal{A}) \|^2 \right] \\
    &= \min_{\mathcal{A}} \mathbb{E}_{\mathbf{x}, \mathcal{S}} \left[ \sum_{j\in\mathcal{S}} \left\| \mathbf{y}_j - \mathbf{A}_j \left(\sum_{i\in\mathcal{S}}\mathbf{A}_i^\top \mathbf{A}_i + \varepsilon \mathbf{I} \right)^{-1} \left(\sum_{i\in\mathcal{S}}\mathbf{A}_i^\top \mathbf{y}_i\right) \right\|^2 \right] \\
    &= \min_{\mathcal{A}} \mathbb{E}_{\mathbf{x}, \mathcal{S}} \left[ \sum_{j\in\mathcal{S}} \left\| \mathbf{A}^\star_j \mathbf{x} - \mathbf{A}_j \left(\sum_{i\in\mathcal{S}}\mathbf{A}_i^\top \mathbf{A}_i + \varepsilon \mathbf{I} \right)^{-1} \left(\sum_{i\in\mathcal{S}}\mathbf{A}_i^\top \mathbf{A}^\star_i \mathbf{x} \right) \right\|^2 \right] \\
    &= \min_{\mathcal{A}} \mathbb{E}_{\mathcal{S}} \left[ \sum_{j\in\mathcal{S}} \left\| \mathbf{A}^\star_j - \mathbf{A}_j \left(\sum_{i\in\mathcal{S}}\mathbf{A}_i^\top \mathbf{A}_i + \varepsilon \mathbf{I} \right)^{-1} \left(\sum_{i\in\mathcal{S}}\mathbf{A}_i^\top \mathbf{A}^\star_i \right) \right\|^2 \right] \\
    &= \min_{\mathcal{A}} \mathbb{E}_{\mathcal{S}} \left[ \sum_{j\in\mathcal{S}} \| \mathbf{A}^\star_j - \mathbf{A}_j \mathbf{K}(\mathcal{S}, \mathcal{A})\|^2 \right]
    \end{aligned}
\end{equation}

Given the above objective functions, upon convergence we are expecting $\mathbf{A}_i = \mathbf{A}_i^\star \mathbf{O}$ and $\mathbf{K}(\mathcal{S}, \mathcal{A}) = \mathbf{O}^\top$.

\weilin{
We need the following hold to make sure the result is independent with sampling $\mathcal{S}$ for some $\mathbf{M}$ (will discuss later on $\mathbf{M}$)
\begin{equation}
    \left(\sum_{i\in\mathcal{S}}\mathbf{A}_i^\top \mathbf{A}_i + \varepsilon \mathbf{I} \right)^{-1} \left(\sum_{i\in\mathcal{S}}\mathbf{A}_i^\top \mathbf{A}^\star_i \right) = \mathbf{M}
    \Leftrightarrow 
    \sum_{i\in\mathcal{S}}\mathbf{A}_i^\top \mathbf{A}^\star_i  = \sum_{i\in\mathcal{S}}\mathbf{A}_i^\top \mathbf{A}_i \mathbf{M}
\end{equation}
which gives us
\begin{equation}
    \sum_{i\in\mathcal{S}} \mathbf{A}_i^\top \left( \mathbf{A}_i^\star - \mathbf{A}_i \mathbf{M}\right) = 0
\end{equation}
The only solution is $\mathbf{A}_i = \mathbf{A}_i^\star \mathbf{M}^{-1}$.
To make our second loss as zero, let first SVD $\mathbf{A}_i^\star$ by $\mathbf{A}_i^\star = \mathbf{U}_i \mathbf{\Sigma}_i \mathbf{V}_i$.
Then,
we want $\mathbf{A}_i \rightarrow \mathbf{U}_i \sqrt{\mathbf{\Sigma}}_i \mathbf{O}$ and $\mathbf{M} \rightarrow \mathbf{O}^\top \sqrt{\mathbf{\Sigma}}_i \mathbf{V}_i$, where $\mathbf{O} \mathbf{O}^\top = \mathbf{I}$.
By combining the results above, we have
\begin{equation}
    \mathbf{A}_i = \mathbf{U}_i \sqrt{\mathbf{\Sigma}}_i \mathbf{O} = \mathbf{A}_i^\star \left( \mathbf{O}^\top \sqrt{\mathbf{\Sigma}}_i \mathbf{V}_i \right)^{-1}
\end{equation}
Therefore, as long as $\mathbf{O}^\top \sqrt{\mathbf{\Sigma}}_i \mathbf{V}_i$ is inversible is ok.
}

\weilin{==================\\}

% Can we have other solutions that has small gradient? No, because ...

\weilin{an orthogonal matrix can rotate or flip a vector space, but it will not stretch it or compress it. For any orthogonal matrix $\mathbf{U}$
\begin{itemize}
    \item Angles are preserved: $\langle \mathbf{U} \mathbf{v}_i, \mathbf{U} \mathbf{v}_j \rangle = \langle \mathbf{v}_i, \mathbf{v}_j \rangle$
    \item Lengths are preserved: $\| \mathbf{U} \mathbf{v} \|_2^2 = \| \mathbf{v}\|_2^2$
    \item Area is preserved, i.e., multiply with orthogonal matrix only rotate or reflect the vector space because $\det(\mathbf{U}) = \pm 1$
\end{itemize}
}

\weilin{====================================\\}
\input{supplementary/archieve/yuandong}
