# Supplementary material for: DyFormer: A Scalable Dynamic Graph Transformer with Provable Benefits on Generalization Ability
Source: arXiv:2111.10447 source file (2023-01-30)
Supplement: Supplementary file 4 [file expressive_power.tex]

\section{Expressive power analysis}

\subsection{}
In the following, we first derives sufficient conditions such that graph Transformers can simulate graph convolutional layer.

\textcolor{red}{
This part should be replace to some most expressive GNN, not normal GNN. 
}
\textcolor{blue}{
Graph convolutional layers are the \textit{de facto} choice for building neural networks that operate on graph structured data. 
Given a node feature matrix $\mathbf{X}\in\mathbb{R}^{N\times d_\text{in}}$, the output of a graph convolutional layer for node $i$ is given by
\begin{equation}
    [\text{GConv}(\mathbf{X})]_{i,:} := \sum_{j \in \mathcal{N}(i)} \alpha_{i,j} \mathbf{X}_{j,:} \mathbf{W} + \mathbf{b},
\end{equation}
where $\mathbf{W} \in \mathbb{R}^{d_\text{in}\times d_\text{out}}$ is the weight matrix, $\mathbf{b} \in \mathbb{R}^{d_\text{out}}$ is the bias vector, and $\alpha_{i,j}$ is the attention weight that propagate from node $j$ to $i$.
}

In the following, we review how self-attention can be adapted from $1$D sequences to graphs.
