# Supplementary material for: DyFormer: A Scalable Dynamic Graph Transformer with Provable Benefits on Generalization Ability
Source: arXiv:2111.10447 source file (2023-01-30)
Supplement: Supplementary file 5 [file hyper_parameter_tuning.tex]

\subsection{Details on baseline hypter-parameters tuning}\label{section:hyper_parameters}

We tune the hyper-parameters of baselines following their recommended guidelines.

\begin{itemize} [noitemsep,topsep=0pt,leftmargin=3mm ]
    \item\textsc{Node2Vec}\footnote{\url{https://github.com/aditya-grover/node2vec}}: We use the default setting as introduced in~\cite{grover2016node2vec}. More specifically, for each node we use $10$ random walks of length $80$, context window size as $10$. The in-out hyper-parameter $p$ and return hyper-parameter $q$ are selected by grid-search in range $\{0.25, 0.5, 1, 2, 5\}$ on the validation set.
    
    \item\textsc{GraphSAGE}\footnote{\url{https://github.com/williamleif/GraphSAGE}}: We use the default setting as introduced in~\cite{hamilton2017inductive}. More specifically, we train two layer GNN with neighbor sampling size $25$ and $10$. The neighbor aggregation is selected by grid-search from ``\text{mean-based aggregation}'', ``\text{LSTM-based aggregation}'', ``\text{max-pooling aggregation}'', and ``\text{GCN-based aggregation}'' on the validation set. 
    In practice, GCN aggregator performs best on Enron, RDS, and UCI, and  max-pooling aggregator performs best on Yelp and ML-10M.
    
    \item\textsc{DynGEM} and \textsc{DynAERNN}\footnote{\url{https://github.com/palash1992/DynamicGEM}}: We use the default setting as introduced in~\cite{goyal2018dyngem} and~\cite{goyal2020dyngraph2vec}. The scaling and regularization hyper-parameters is selected by grid-search in range $\alpha \in \{ 10^{-6}, 10^{-5}\}$, $\beta \in \{0.1, 1, 2, 5\}$, and $\nu_1,\nu_2 \in \{10^{-6}, 10^{-4}\}$ on the validation set.
    
    \item\textsc{DySAT}\footnote{\url{https://github.com/aravindsankar28/DySAT}}: We use the default setting and model architecture as introduced in~\cite{sankar2018dynamic}. The co-occurring positive node pairs are sampled by running 10 random walks of length 40 for each node. The negative sampling ratio is selected by grid-search in the range $\{0.01, 0.1, 1\}$, number of the self-attention head is selected in the range $\{8, 16\}$, and the feature dimension is selected in the range $\{128, 256\}$ on the validation set.
    
    \item\textsc{EvolveGCN}\footnote{\url{https://github.com/IBM/EvolveGCN}}: We use the default setting and model architecture as introduced in~\cite{pareja2020evolvegcn}. We train both EvolveGCN-O and EvolveGCN-H and report the architecture with the best performance on the validation set. In practice, EvolveGCN-O performs best on UCI, Yelp, and ML-10M, EvolveGCN-H performs best on Enron and RDS.
\end{itemize}
% \footnote{For \textsc{GraphSAGE}, GCN aggregator performs best on Enron, RDS, and UCI, and  max-pooling aggregator performs best on Yelp and ML-10M. For EvolveGCN, EvolveGCN-O performs best on UCI, Yelp, and ML-10M, EvolveGCN-H performs best on Enron and RDS.} 

\subsection{Additional details on experiment configuration}\label{section:our_config}

We select a single set of hyper-parameters for each dataset using grid search. 
More specifically, we select the negative sampling ratio (i.e., number of positive edge/number of negative edge) in the range $\{0.01, 0.1, 1\}$, number of the self-attention head is selected in the range $\{8, 16\}$, feature dimension is selected in the range $\{128, 256\}$, number of layers in the range $\{2, 4, 6\}$, maximum shortest path distance $D_{\max}$ in the range $\{2, 3, 5\}$ on the validation set, and the hyper-parameter that balances the importance of two pre-taining tasks $\gamma=1$. 
The hyper-parameter for each dataset is summarized in Table~\ref{table:hyper_parameters}.
 
\begin{table}[h]
\caption{Hyper-parameters used in \DGT for different datasets. ``-'' stands for hyper-parameters that are not required.} \label{table:hyper_parameters}
\centering
\begin{tabular}{lccccccc}
\hline\hline
                                          & \textbf{Enron} & \textbf{RDS} & \textbf{UCI} & \textbf{Yelp} & \textbf{ML-10M} & \textbf{Wiki} & \textbf{Reddit} \\ \hline\hline
\text{Self-attention head}              &  $16$           & $16$           & $8$          & $8$           & $8$             & $8$                & $8$             \\ \hline
\text{Hidden dimension}                 &  $256$          & $256$          & $128$        & $128$         & $128$           & $128$              & $128$           \\ \hline
\text{Number of layer}                  &  $2$            & $2$            & $6$          & $4$           & $4$             & $2$                & $2$             \\ \hline
\text{Hidden feature dropout out ratio} &  $0.5$          & $0.5$          & $0.5$        & $0.5$         & $0.5$           & $0.5$              & $0.5$           \\ \hline
\text{Self-attention dropout ratio}     &  $0.1$          & $0.1$          & $0.1$        & $0.5$         & $0.5$           & $0.1$              & $0.1$           \\ \hline
\text{Negative sampling ratio}          &  $50$           & $10$           & $10$         & $10$          & $10$            & $-$               & $-$            \\ \hline
\text{Maximize shortest path distance}  &  $5$            & $5$            & $5$          & $5$           & $5$             & $5$                & $5$             \\ \hline
\text{Mini-batch size}                  &  $512$          & $512$          & $512$        & $512$         & $512$           & $800$              & $800$           \\ \hline\hline
\end{tabular}
\end{table}

During training, we set the target node size as the largest number our GPU (Nvidia RTX $3090$) can fit, and sample the context nodes the same size as target nodes. In practice, we found that a mini-batch size of $512$ works well on all datasets.
During the evaluation, we set all validation and testing nodes as target nodes during evaluation. Notice that since gradients are not required during evaluation, therefore we can obtain all the self-attention values by first splitting all self-attentions into multiple chunks, then we iterative compute the self-attention in each chunk on GPU as shown in Figure~\ref{fig:evaluation_full_gradient}. Since every iteration only a fixed number of self-attention are computed and computing the self-attention is the most memory-consuming operation, \DGT can inference validation and testing set of any size.

\begin{figure}[h]
    \centering
    \includegraphics[width=0.95\textwidth]{figures/evaluation_full_gradient.pdf}
    \caption{Suppose we want to compute the pairwise self-attention between nodes $\{v_1,\ldots, v_5\}$. We can first split all self-attentions into multiple chunks, and iteratively compute the self-attention value in each chunk. For example, at the first iteration, we first compute the self attention between node $\{v_1,\ldots, v_3\}$ (in blue) and store it in memory (in yellow). Then, at the second iteration, we compute the attention between node $\{v_1,\ldots, v_3\}$ and node $\{v_4,v_5\}$.}
    \label{fig:evaluation_full_gradient}
\end{figure}
