# Supplementary material for: DyFormer: A Scalable Dynamic Graph Transformer with Provable Benefits on Generalization Ability
Source: arXiv:2111.10447 source file (2023-01-30)
Supplement: Supplementary file 6 [file compare_diff_trans.tex]

\section{Comparison of different graph Transformer} \label{section:diff_graph_trans_appendix}

In this section, we provide details on the comparison of different graph Transformers as summarized in Table~\ref{table:compare_diff_graph_trans}, provide detailed information on different positional encoding type in Section~\ref{section:diff_pos_enc}, and discussion on othe application of graph Transformers in Section~\ref{section:graph_trans_other_app}. 
% Graphormer, Graphsfromer, GraphBert, 

% mini-batch sampling, support dynamic graph?, positional encoding, 


\begin{table}[h]
\centering
\caption{Comparison of different graph Transformers.} \label{table:compare_diff_graph_trans}
\scalebox{0.9}{
\begin{tabular}{lllll}
\hline\hline
\text{Method}       & \textsc{Graphormer} & \textsc{GraphTransformer} & \textsc{GraphBert} & \DGT (ours)\\ \hline\hline
\text{Mini-batch}      & No                  & No                    & Yes                & Yes\\ \hline
\text{Graph type}      & Static              & Static                & Static             & Dynamic \\ \hline
\text{Attention type}  & Full-attention      & $1$-hop attention     & Full-attention     & Full-attention \\ \hline
\multirow{3}{*}{Encoding type}   & Centrality Encoding &                        & WL-based    & Temporal Connection   \\ % \cline{2-5} 
                                 & Spatial Encoding    & Laplacian Eigenvector  & Intimacy-based & Spatial Distance  \\ % \cline{2-5} 
                                 & Edge Encoding       &                        & Hop-based        &                \\ \hline\hline
\end{tabular}
}
% \vspace{-10pt}
\end{table}


% \multirow{2}{*}{Method}
% \noindent\textbf{Positional encoding types.~}
\subsection{Positional encoding types}\label{section:diff_pos_enc}
In the following, we summarize the positional encoding of different methods.

($1$) \textsc{Graphormer}~\citep{ying2021transformers}:
\begin{itemize} [noitemsep,topsep=0pt,leftmargin=5mm ]
    \item Centrality Encoding: the in-degree and out-degree information of each node. Then, they add the degree information to the original node feature.
    \item Spatial Encoding: shortest path distance between two nodes. Then, they add the shortest path distance as a bias term to the self-attention.
    \item Edge Encoding: the summation of all egde features on the shortest path. Then, they add the shortest path distance as a bias term to the self-attention.
\end{itemize}

($2$) \textsc{GraphTransformer}~\citep{dwivedi2020generalization} proposes to use the Laplacian Eigenvectors. Then, they add the Eigenvectors to the original node feature.

($3$) \textsc{GraphBert}~\citep{zhang2020graph}:
\begin{itemize} [noitemsep,topsep=0pt,leftmargin=5mm ]
    \item Weisfeiler-Lehman Absolute Role Embedding: the node label generated by the Weisfeiler-Lehman (WL) algorithm according to the structural roles of each node in the graph data. Then, they add the labelled node information to the original node feature.
    \item Intimacy based Relative Positional Embedding:  the placement orders of the serialized node list ordered by the Personalized PageRank score of each node.  Then, they add the node order information to the original node feature.
    \item Hop based Relative Distance Embedding: shortest path distance between a node to the center node of the sampled subgraph. Then, they add the shortest path distance as a bias information to the original node feature.
\end{itemize}


\subsection{Graph Transformer with other applications} \label{section:graph_trans_other_app}
% On the other hand,
Transformers are also applied to other graph types or downstream tasks. 
For example, \textsc{HGT}~\cite{hu2020heterogeneous} and \textsc{GTNs}~\cite{yun2019graph}
propose a first-order graph transformer to solve the heterogeneous graph representation learning problem, 
\textsc{TagGen}~\cite{zhou2020data} is working on synthetic graph generation problems, which are out of the scope of this paper.
